# Supplementary material for: Correlative Imaging of Individual CsPbBr3 Nanocrystals: Role of Isolated Grains in Photoluminescence of Perovskite Polycrystalline Thin Films
Source: arXiv:2304.05114 source file (2023-05-09)
Supplement: Supplementary file 1 [file Supporting_info.pdf]

# Supporting information: Correlative Imaging of Individual CsPbBr<sub>3</sub> Nanocrystals: Role of Isolated Grains in Photoluminescence of Perovskite Polycrystalline Thin Films

Petr Liška,<sup>\*,†,‡</sup> Tomáš Musálek,<sup>†</sup> Tomáš Šamořil,<sup>†,‡,§</sup> Matouš Kratochvíl,<sup>¶</sup>  
Radovan Matula,<sup>†</sup> Michal Horák,<sup>†,‡</sup> Matěj Nedvěd,<sup>†</sup> Jakub Urban,<sup>†</sup> Jakub Planer,<sup>‡</sup>  
Katarína Rovenská,<sup>‡</sup> Petr Dvořák,<sup>†,‡</sup> Miroslav Kolíbal,<sup>†,‡</sup> Vlastimil Křápek,<sup>†,‡</sup>  
Radek Kalousek,<sup>†</sup> and Tomáš Šikola<sup>†,‡</sup>

<sup>†</sup>*Institute of Physical Engineering, Faculty of Mechanical Engineering, Brno University of Technology, Technická 2896/2, 616 69 Brno, Czech Republic*

<sup>‡</sup>*Central European Institute of Technology, Brno University of Technology, Purkyňova 123, 612 00 Brno, Czech Republic*

<sup>¶</sup>*Faculty of Chemistry, Brno University of Technology, Purkyňova 464/118, 612 00 Brno, Czech Republic*

<sup>§</sup>*TESCAN ORSAY HOLDING, a.s, Libušina tř. 21, Brno 623 00, Czech Republic*

E-mail: petr.liska1@vutbr.cz

## S1: Electronic and structural properties of CsPbBr<sub>3</sub> NCs

To predict the influence of the CsPbBr<sub>3</sub> NCs' morphology on their PL properties, we have built a quantum confinement model based upon high-resolution TEM measurements and effective mass theory with parameters obtained by DFT. Figure S1a displays atomic-resolution TEM images of the CsPbBr<sub>3</sub> NCs (see Supporting Info S2), measured in order to obtain the lattice parameter of the NCs. The atomic-resolution images of CsPbBr<sub>3</sub> NCs were then processed by 2D fast Fourier transform (2D FFT), shown in Figure S1b in order to determine the lattice constant. To determine the experimental value of the CsPbBr<sub>3</sub> band gap, electron energy loss spectroscopy (EELS) measurements took place (Figure S1c), which indicated the band gap of CsPbBr<sub>3</sub> to be  $E_{g,e} = (2.3 \pm 0.1)$  eV. The experimentally obtained lattice parameters from several NCs were displayed in a histogram (Figure S1d) which was fitted by a normal distribution. The statistically determined value of the lattice parameter was determined to be  $\tilde{a} = (5.9 \pm 0.1)$  Å which is in good agreement with the value reported in the literature  $a = 5.865$  Å.<sup>1</sup>

Figure S1e displays DFT calculated free energies as the function of the unit cell volume, and a fit to the Murnaghan equation of states (see Methods). The equilibrium lattice constant of CsPbBr<sub>3</sub> is found to be  $a_0 = 5.92$  Å, which agrees well with the experiment. Figure S1f displays the band structure of bulk CsPbBr<sub>3</sub> calculated by DFT (see Methods) with equilibrium lattice constant as an input. Due to the nature of the DFT calculations, which artificially reduce the value of the band gap, the theoretical value of band gap was falsely determined as  $E_{g,t} = 2.01$  eV. For the purpose of the QCE model in this paper, we have used the measured value of the band gap by EELS  $E_{g,e} = (2.3 \pm 0.1)$  eV as a starting point for our simulations. By fitting the experimental data of the PL peak emission of individual NCs by eq. (1), the band gap was determined as  $E_g = (2.345 \pm 0.002)$  eV. From the band structure, the electron and hole effective masses  $m_e^* = 0.177 m_e$ ,  $m_h^* = -0.187 m_e$  in the direction  $\Gamma$ -R were obtained, where  $m_e$  is the mass of a free electron (see Methods). These values are in good agreement with Ref.,<sup>2</sup> however, the incorrect value of the band gap suggests that these

effective masses can vary by order of several per cent.

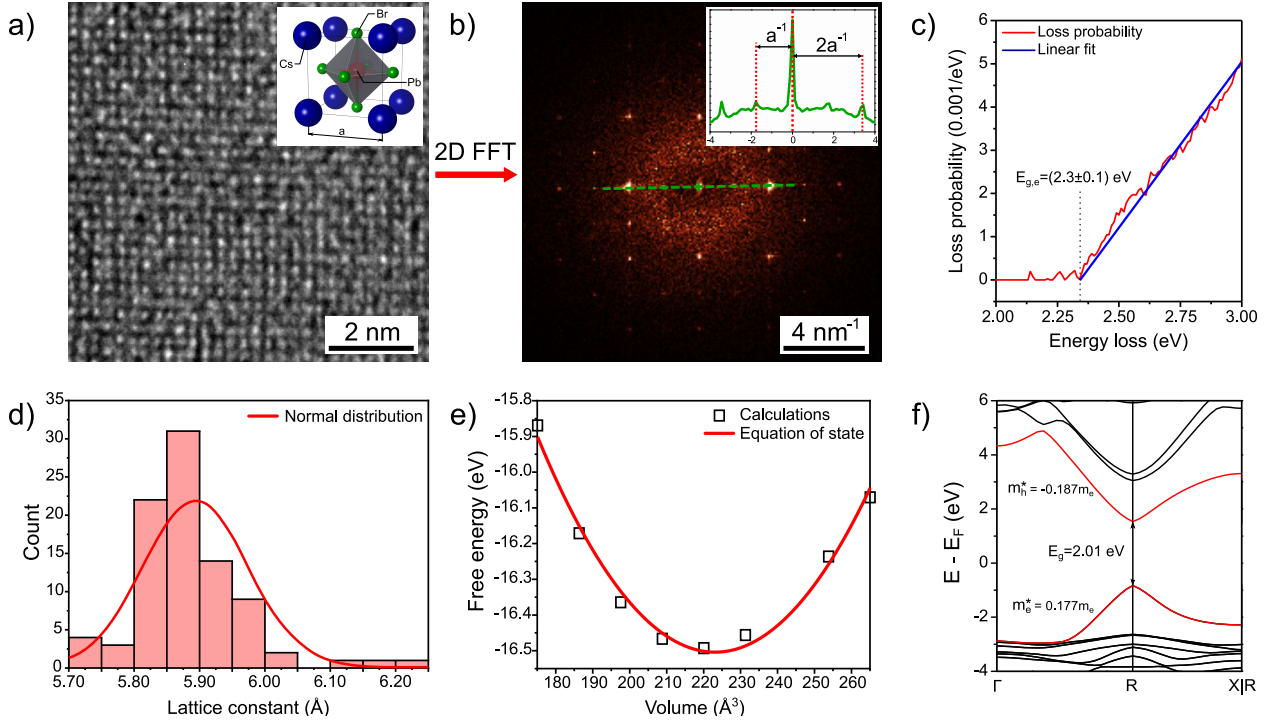

Figure S1: a) Atomic-resolution TEM image of the analysed CsPbBr<sub>3</sub> NC with the model of the CsPbBr<sub>3</sub> cubic lattice. The high-resolution images post-processed in programme Gwyddion<sup>3</sup> via 2D-FFT to acquire the experimental lattice constant  $a$ . c) EELS loss probability spectrum of the CsPbBr<sub>3</sub> NCs with band gap determined experimentally as  $E_{g,e} = (2.3 \pm 0.1) \text{ eV}$ . d) A histogram of lattice constants determined for 53 distinct CsPbBr<sub>3</sub> NCs fitted by normal distribution with the value of experimental lattice parameter  $a = (5.9 \pm 0.1) \text{ \AA}$ . e) Volume relaxation calculations utilizing the experimental lattice parameter  $a$  as a starting point, fitted by Murnaghan equation of state with an outcome of theoretical equilibrium lattice parameter  $a_0 = 5.92 \text{ \AA}$ . f) The theoretically calculated band structure of bulk crystal CsPbBr<sub>3</sub> acquired via DFT with an input parameter of theoretical equilibrium lattice parameter and output parameters of electron and hole effective masses for effective mass modelling of CsPbBr<sub>3</sub> NCs' PL response.

## S2: Sensitivity of CsPbBr<sub>3</sub> nanocrystals to FIB and electron beam in TEM

The exposure to the required dose of Ga ions during the fabrication of FIB micro-markings decreases the PL integral intensity by about 6 % (Figure S2) but does not alter the PL peak emission wavelength or FWHM.

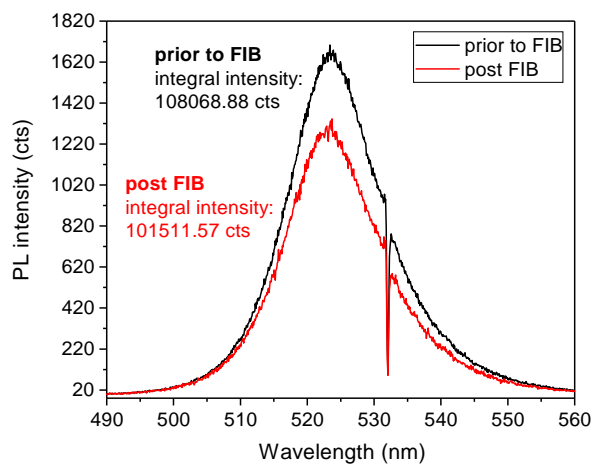

Figure S2: Prior to FIB processing and post FIB processing obtained typical PL integral intensities of CsPbBr<sub>3</sub> NC.

Due to the intense destruction of CsPbBr<sub>3</sub> NCs during the TEM analysis (Figure S3a), which resulted in the incapability of atomic-resolution images nor diffraction patterns, a compromise needed to be made. The acquisition of the TEM and EELS measurements has been made on the colloidal CsPbBr<sub>3</sub> NCs, which should exhibit the same crystalline structure as the CsPbBr<sub>3</sub> NCs prepared by drop casting. The STEM overview image of the colloidal nanocrystals is displayed in Figure S3b. The challenges of the CsPbBr<sub>3</sub> NCs and thin films imaging have been already discussed in<sup>4,5</sup> which results are in agreement with our observations.

### S3: Stoichiometry of CsPbBr<sub>3</sub> nanocrystals

To determine the purity of the prepared CsPbBr<sub>3</sub> NCs, integral XPS was done on the ensemble of the characterized NCs (Figure S4). The resulting stoichiometry was determined as Cs<sub>1.2</sub>Pb<sub>1</sub>Br<sub>2.8</sub>.

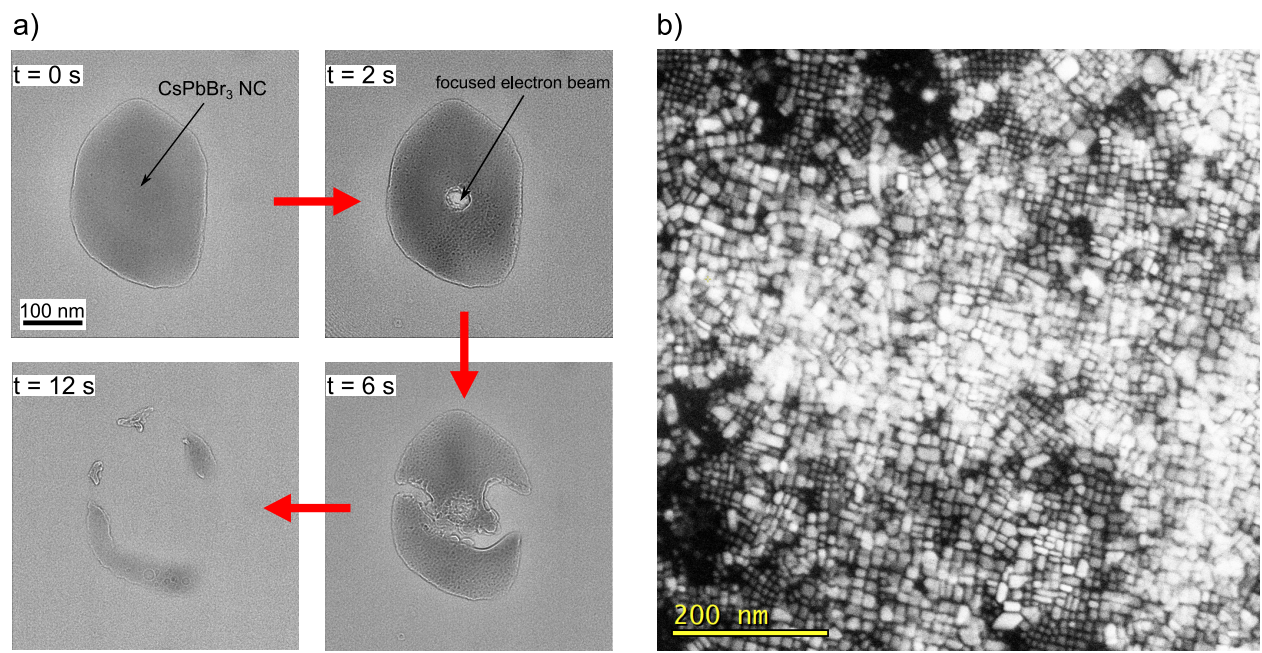

Figure S3: a) Immediate degradation of drop casted CsPbBr<sub>3</sub> NCs in TEM observation under focused electron beam. b) Overview STEM image of colloidal CsPbBr<sub>3</sub> NCs serving for the crystal lattice acquisition.

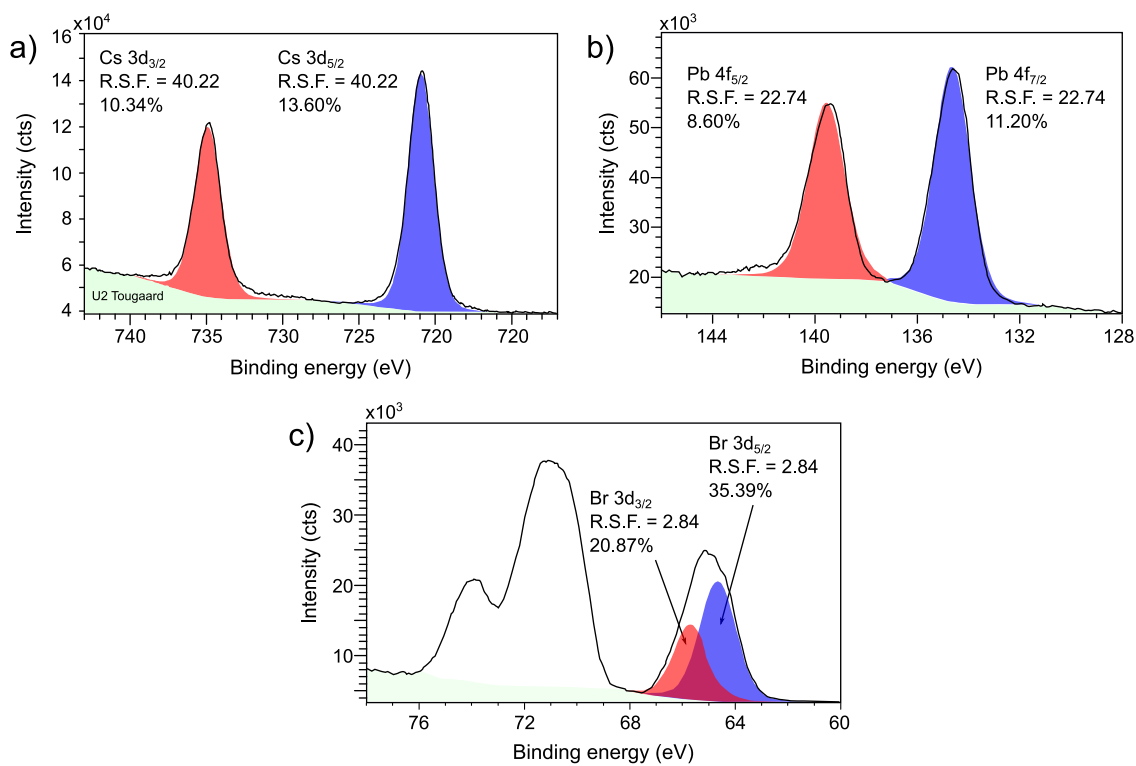

Figure S4: XPS spectra for determination of the stoichiometry of a) Cs, b) Pb, and c) Br atoms.

## S4: Error of the spheroidal approximation

In order to estimate the error of the used spheroid approximation of the CsPbBr<sub>3</sub> NCs, the effective length  $a$  and height  $c$  of the NC have been compared to the lengths and heights of the inscribed  $a_{\text{in}}, c_{\text{in}}$  (Figure S5a) and circumscribed  $a_{\text{out}}, c_{\text{out}}$  (Figure S5b) spheroid. The effective lengths  $a$  have been acquired from each NC by averaging over 12px from the horizontal profile in SEM and effective heights  $c$  have been acquired by averaging over 12px from the topography of individual NC in the program Gwyddion.<sup>3</sup> The lengths and heights of the inscribed or circumscribed spheroid were obtained by fitting the spheroid inside the NC or fitting the spheroid so it would contain the whole NC respectively. Figure S5 displays the comparison between the a) inscribed or b) circumscribed lengths and heights of the NCs with the effective values. The average difference between the values for inscribed NCs and effective values was overall bigger than in the case of the circumscribed spheroid approximation, hence, the circumscribed spheroid approximation was used. The average deviation of the used values and the effective ones was determined ranging between 5 – 20 %.

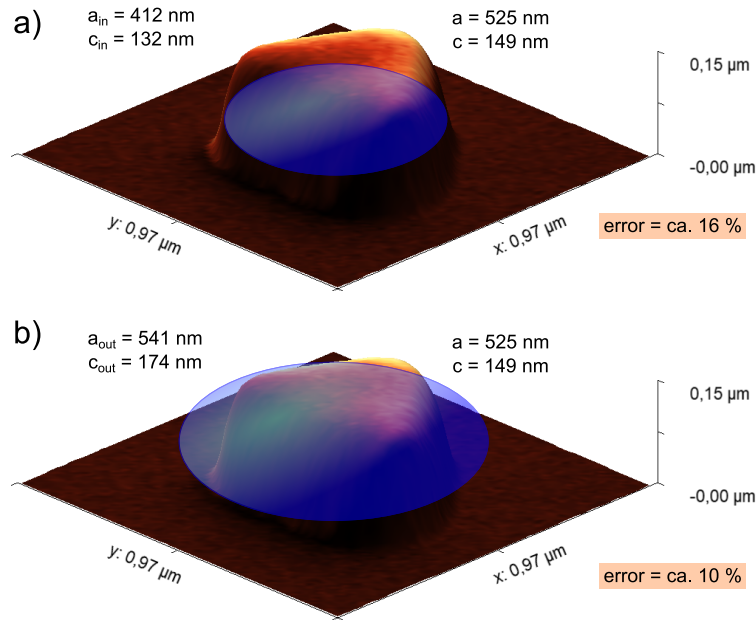

Figure S5: a) Inscribed and b) circumscribed spheroid compared to the effective length and height of the NC.

## References

- (1) Mehl, M. J.; Hicks, D.; Toher, C.; Levy, O.; Hanson, R. M.; Hart, G.; Curtarolo, S. The AFLOW Library of Crystallographic Prototypes. *Computational Materials Science* **2017**, *136*, S1–S828.
- (2) Becker, M. A.; Vaxenburg, R.; Nedelcu, G.; Sercel, P. C.; Shabaev, A.; Mehl, M. J.; Michopoulos, J. G.; Lambrakos, S. G.; Bernstein, N.; Lyons, J. L. et al. Bright triplet excitons in caesium lead halide perovskites. *Nature* **2018**, *553*, 189–193.
- (3) Nečas, D.; Klapetek, P. Gwyddion: an open-source software for SPM data analysis. *Central European Journal of Physics* **2012**, *10*, 181–188.
- (4) Brennan, M.; Kuno, M.; Rouvimov, S. TEM Analysis of CsPbBr<sub>3</sub> Nanocrystals. *Microscopy and Microanalysis* **2017**, *23*, 2096–2097.
- (5) Duong, T. M.; Sharma, K.; Agnese, F.; Rouviere, J.-L.; Okuno, H.; Pouget, S.; Reiss, P.; Ling, W. L. Practice of electron microscopy on nanoparticles sensitive to radiation damage. *Frontiers in Chemistry* **2022**, *10*.
